# Supplementary material for: Low-Rank+Sparse Tensor Compression for Neural Networks
Source: arXiv:2111.01697 source file (2021-11-02)
Supplement: Supplementary file 1 [file appendix.tex]

\section{Appendix}
